# Supplementary material for: DiffSurf: A Transformer-based Diffusion Model for Generating and Reconstructing 3D Surfaces in Pose
Source: arXiv:2408.14860 source file (2024-08-27)
Supplement: Supplementary file 1 [file supplemental.tex]

\title{DiffSurf: A Transformer-based Diffusion Model for \\  Generating and Reconstructing 3D Surfaces in Pose} 

% TODO REVIEW: If the paper title is too long for the running head, you can set
% an abbreviated paper title here. If not, comment out.
\titlerunning{DiffSurf}

% TODO FINAL: Replace with your author list. 
% Include the authors' OCRID for the camera-ready version, if at all possible.
\author{Yusuke Yoshiyasu\inst{1}\orcidlink{0000-0002-0433-9832} \and
Leyuan Sun\inst{1}\orcidlink{0000-0001-6123-9339}}

% TODO FINAL: Replace with an abbreviated list of authors.
\authorrunning{Y.Yoshiyasu and L. Sun}
% First names are abbreviated in the running head.
% If there are more than two authors, 'et al.' is used.

% TODO FINAL: Replace with your institution list.
\institute{National Institute of Advanced Industrial Science and Technology (AIST), 1-1-1 Umezono, Tsukuba, Japan 
\email{\{yusuke-yoshiyasu,son.leyuansun\}@aist.go.jp}}

\begin{comment}
    
\makeatletter
\let\@oldmaketitle\@maketitle% Store \@maketitle
\renewcommand{\@maketitle}{\@oldmaketitle% Update \@maketitle to insert..
\centering
\vspace{-20pt}
  \includegraphics[width=1\textwidth]{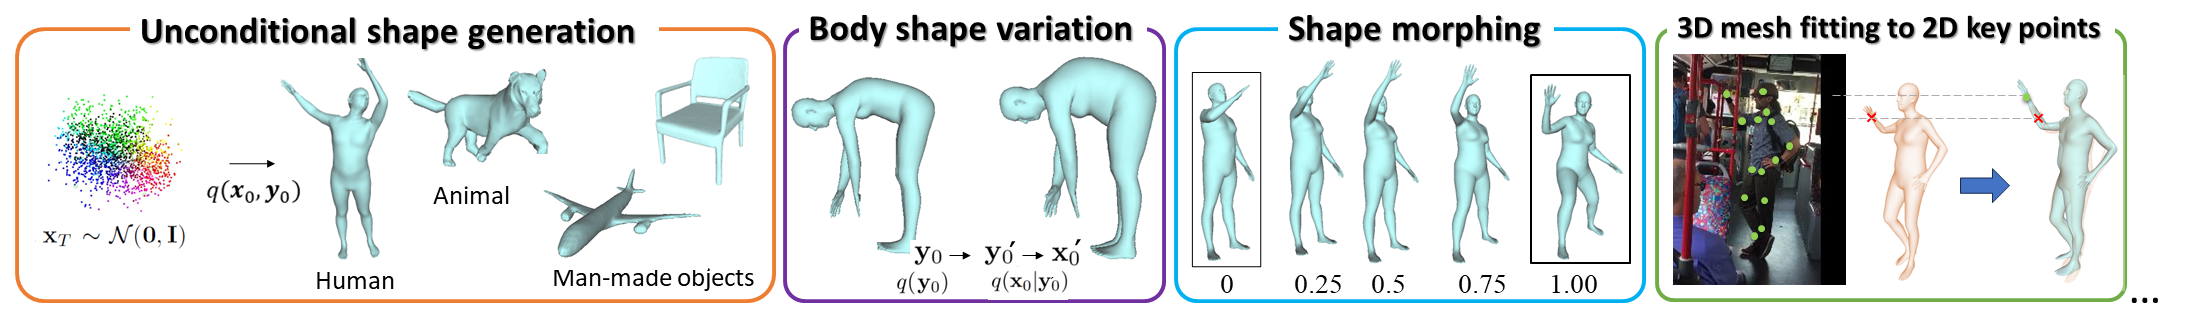}
  \vspace{-10pt}
  \captionof{figure}{DiffSurf handles various tasks including 3D mesh generation, editing and fitting to 2D key points. }
  \vspace{10pt}
  \label{fig:teaser}
}
\makeatother

\end{comment}

\maketitle

\begin{figure*}[h]
\begin{center}
 \includegraphics[width=\linewidth]{images/supplemental/shapenet13.png}
 \caption{Class-conditioned generation results of ShapeNet 13 objects with DiffSurf: Airplane, Bench, Cabinet, Car, Chair, Display, Lamp, Loud speaker, Rifle, Sofa, Table, Telephone, Watercraft. DiffSurf can generate 3D surfaces of diverse objects. }
 \label{fig:shapenet13}
\end{center}
\end{figure*}

\begin{figure}[b]
\begin{center}
 \includegraphics[width=0.8\linewidth]{images/rebutttal/failure.png}
 \caption{Failure cases. Left: Distortions on extreme poses. Right: Self-intersections of body parts. }
 \label{fig:failures}
\end{center}
\end{figure}

\section{Appendix: Failure cases and limitations }

With 230K training meshes, DiffSurf rarely generates results that exhibit  artifacts on extreme poses (Fig. \ref{fig:failures} left)  but more cases are found in less data settings (Fig. \ref{fig:dataset_scale}). Self-intersections of the body parts occur sometimes (Fig. \ref{fig:failures} right). %Currently, like most of other 3D generative models, our method is limited to category-level generation, except on Animal3D dataset (40 species).%, where its categorical diversity determined by the dataset trained on.  

While DiffSurf implicitly considers body shapes and poses as distinct variables, by introducing mesh and body joint tokens that are  treated as distinct modalities, it does not explicitly establish disentangle representation of body shape and pose. Thus,  during pose-conditional mesh generation  we occasionally found that the body shape changes according to the pose change. Likewise, male/female is not entirely consistent across all frames during body shape variation, as it can be seen from Fig. \ref{fig:more_body_shape}. A  method for establishing disentangled representation of body shape/pose and controlling a body model based on attributes would be a useful tool in applications that require precise controls over body shape/pose and body styles.

\begin{table}[t]
%\captionsetup[subtable]{justification=centering}
\caption{Comparisons with SOTA methods on unconditional generation of Car and Chair.}
\centering
\subcaption{ShapeNet validation set from \cite{pointflow}}
\vspace{-5pt}
\scalebox{0.8}[0.8]{
\begin{tabular}{c c c c c c c }
\hline 
&  \multicolumn{3}{c}{Car} & \multicolumn{3}{c}{Chair}   \\
 & MMD-CD $\downarrow$ & COV-CD [\%] $\uparrow$ & 1-NNA-CD [\%] $\downarrow$ & MMD-CD $\downarrow$ & COV-CD [\%] $\uparrow$ &  1-NNA-CD [\%] $\downarrow$ \\
\hline 
LION \cite{zeng2022lion} &  1.06 & 42.6 &  68.6 &  3.95 & 45.7 &  57.7 \\
SLIDE \cite{slide2023} & 1.10 &  35.2 & 81.8 & 3.84 & 46.9 & 59.8 \\
Ours & 1.18 &  39.2 &  85.5 & 4.06 & 43.6 &  59.7 \\ 
\hline 
\label{tab:quantitative1}
\end{tabular}
}
\vspace{20pt}
\subcaption{ShapeNet validation set from \cite{Peng2021SAP}}
\vspace{-5pt}
\centering
\scalebox{0.8}[0.8]{
\begin{tabular}{c c c c c c c}
\hline 
&  \multicolumn{3}{c}{Car} & \multicolumn{3}{c}{Chair} \\
& MMD-CD $\downarrow$ & COV-CD [\%] $\uparrow$ & 1-NNA-CD [\%] $\downarrow$ & MMD-CD $\downarrow$ & COV-CD [\%] $\uparrow$ &  1-NNA-CD [\%] $\downarrow$ \\
\hline 
TreeGAN & --- & 33.2 & 91.3 & --- & 49.6 & 70.2 \\
ShapeGF & --- & 44.7 &  67.2 & --- & 52.8 &  56.5 \\
PVD & --- & 40.0 & 70.0 & --- & 48.1 & 55.3 \\
DPM & --- & 33.2 & 86.3 & --- & 44.0 & 66.1 \\
SPGAN & --- &  32.5 & 85.1 & --- & 30.1 & 79.0 \\
LION \cite{zeng2022lion} & 1.22 & 25.2 & 72.8 & 3.63 & 47.4 & 53.9 \\
SLIDE \cite{slide2023} & 1.04 & 40.5 &  61.4 & 3.59 &  48.6 &  56.7 \\
Ours &  1.13  & 36.3  & 66.2 & 3.86 & 43.3 & 58.4 \\
\hline 
\label{tab:quantitative2}
\end{tabular}
}
\end{table}

\begin{figure*}[t]
\begin{center}
 \includegraphics[width=\linewidth]{images/supplemental/vs_lion.png}
 \caption{Qualitative comparison with LION \cite{zeng2022lion} on unconditional generation of chairs.  }
 \label{fig:vs_lion}
\end{center}
\end{figure*}

\section{Appendix: Comparison with SOTA 3D shape diffusion models }

In Table \ref{tab:quantitative1} and \ref{tab:quantitative2}, we show the quantitative comparisons with the state-of-the-art (SOTA) 3D shape generation techniques. We reproduced LION \cite{zeng2022lion} and SLIDE \cite{slide2023} using the source codes, pre-trained models and generated samples made available by the authors. The evaluation metric scores of TreeGAN \cite{9009495}, ShapeGF \cite{ShapeGF}, PVD \cite{Zhou_2021_ICCV}, DPM \cite{luo2021diffusion} and SPGAN \cite{SP-GAN} taken from \cite{slide2023} are also presented in Table \ref{tab:quantitative2} as a supplementary reference, although their evaluation settings may not be the same as our experiments.  We tested on the two different validation sets from \cite{pointflow} and \cite{Peng2021SAP}. Note that LION is trained on the training set from \cite{pointflow}, whereas SLIDE is trained on the dataset provided by \cite{Peng2021SAP}. The three standard evaluation metrics are used to evaluate the quality of surface generation results, which are the minimum matching distance (MMD), coverage score (COV) and 1-NN classifier accuracy (1-NNA). These metric scores are calculated using Chamfer distances \cite{pointflow}. To evaluate the quality of generated 3D surface instead of point clouds, we sample 2048 points uniformly from generated meshes after applying Shape-As-Points (SAP) \cite{Peng2021SAP}. The meshes are normalized to [-1,1] before calculating the metrics.  

Overall, DiffSurf is comparable to LION \cite{zeng2022lion} and SLIDE \cite{slide2023} according to the evaluation metric scores listed in Table \ref{tab:quantitative1} and \ref{tab:quantitative2}. A notable difference can be found in the Car cases where the LION's metric scores differ from the others by large margins, implying that the two validation sets have slightly different data distributions and currently these models trained on a relatively small class-level dataset are not able to always generalize well to the data distribution different from the training dataset.

% Qualitative comparison against LION
In Fig. \ref{fig:vs_lion}, we qualitatively compared the results generated by DiffSurf and LION \cite{zeng2022lion}. These meshed results were obtained through the same post process based on the SAP models provided by SLIDE \cite{slide2023} which are trained with no synthetic noise augmentation (the models are referred to as "symmetry" for LION and "normal\_symmetry" for DiffSurf). As DiffSurf incorporates surface normals in the diffusion process and provide them to SAP as additional input, the generated surfaces are visually more pleasing than those generated by LION. DiffSurf also leverages the ability of diffusion transformers which show strong generation performances by exploiting long-range dependencies between points, thereby removing the need of hierarchical architecture as in LION and making it faster than LION. As noted in \cite{zeng2022lion}, in order to generate meshes in good quality by LION, a careful fine-tuning process of the SAP model is required to adapt to its relatively noisy point cloud generation results (without surface normals), even though LION employs the additional secondary diffusion model to refine the generated point clouds. 

Even though it utilizes two latent diffusion models as in LION, SLIDE is more efficient than LION as its latent diffusion models operate on sparse latent points, not on point clouds. In addition, sparse latent points enables controllable mesh generation such as shape combination. On the other hand, DiffSurf can generate a wider range of objects than SLIDE as shown in Fig \ref{fig:shapenet13}. This is because DiffSurf's general transformer architecture allows us to easily build and train a class-conditioned generation model that accommodates dozens of objects, by slightly changing its diffusion transformer configuration to input class labels as tokens. In contrast, the hierarchical and sequential nature of SLIDE's network architecture, which needs to train an auto-encoder and two DDPMs for each category, faces difficulties when one wants to increase the number of object classes to generate.

\begin{figure}[t]
\begin{center}
 \includegraphics[width=\linewidth]{images/supplemental/architecture.png}
 \caption{The network architecture of DiffSurf. (a) Diffusion transformer. (b) Upsampler for human generation (fixed connectivity). (c) Upsampler for generating man-made objects. }
 \label{fig:diffsurf_arch}
\end{center}
\end{figure}

\section{Appendix: Details on DiffSurf architecture}

DiffSurf is a diffusion model for generating, editing and reconstructing 3D surfaces based on a plain transformer model, which is easily generalizable and extendable to accommodate a wide range of object types. Figure \ref{fig:diffsurf_arch} illustrates the network architecture of DiffSurf which consists of a diffusion transformer and up-sampler. 

% transformer
\noindent{\bf Diffusion transformer } The inputs to the diffusion transformer consist of noisy 3D coordinates and other geometric attributes of a set of joint query tokens $Q_{\rm J}=\{ Q^1_{\rm J} \ldots Q^J_{\rm J} \} $, corresponding to a skeleton with $J$ body joints, and  a set of coarse vertex query tokens $Q_{\rm V}= \{ Q^1_{\rm V} \ldots Q^N_{\rm V} \} $, corresponding to a surface mesh comprising $N$ vertices.

We denote the input noisy 3D coordinates and $D$-dimensional attributes of surface vertices, body joints and their concatenations are respectively denoted as ${\bf x}_t \in \mathbb{R}^{N \times (3 + D)}$, ${\bf y}_t \in \mathbb{R}^{J \times (3 + D)}$ and ${\bf X}_t \in  \mathbb{R}^{(J + N) \times (3 + D)}$, respectively. The diffusion transformer processes these two modalities of data and their corresponding timesteps $t_x$ and $t_y$ as tokens. It outputs noise predictions for vertices and joints, $\epsilon_\theta^x$ and $\epsilon_\theta^y$. Our diffusion transformer consists of $L$ layers of transformer blocks and input/output MLP layers. Each transformer block has hidden layers with $d$ channels. The input MLP layer converts ${\bf x}_t$ and ${\bf y}_t$ into $d$-dimensional transformer embedding features and the output MLP layer converts the transformer-processed features into $\epsilon_\theta^x$ and $\epsilon_\theta^y$.

For human generation, we input the noisy 3D coordinates of vertices ${\bf x}_t \in \mathbb{R}^{431 \times 3}$ and joints ${\bf y}_t \in \mathbb{R}^{14 \times 3}$ to the diffusion transformer. These are first fed into the input MLP layer and concatenated with the time embeddings. Then we have an embedding feature ${\bf f}_t \in \mathbb{R}^{(2 + 14 + 431) \times 256}$ that is iteratively processed by the transformer blocks. After dropping the time embedding tokens of the transformer features, the output MLP layer converts the features back  into 3D to predict noise i.e. $\epsilon_\theta^x \in \mathbb{R}^{431 \times 3}$ and  $\epsilon_\theta^y \in \mathbb{R}^{14 \times 3}$.    

For the generation of man-made objects, we concatenate the noisy 3D coordinates of vertices (2048 points) and the corresponding surface normals ${\bf n}_t \in \mathbb{R}^{2048 \times 3}$ to construct a noisy input: ${\bf x}_t \in \mathbb{R}^{2048 \times 6}$. The rest of the process proceeds in a same manner as the human generation case as shown in Fig. \ref{fig:diffsurf_arch} (a).  

% upsamplers
\noindent{\bf Up-sampling } After a coarse mesh comprising $N$ vertices, ${\bf v} \in \mathbb{R}^{N \times 3} $ and corresponding surface normals ${\bf n} \in \mathbb{R}^{N \times 3} $ are obtained from the noise prediction $\epsilon^x_\theta$ by the diffusion transformer, we optionally apply an upsampling operation. The upsamplers used in the generations of humans/animals, where the connectivity of the mesh is fixed, and man-made objects differ in their structures as shown in Fig. \ref{fig:diffsurf_arch} (b) and (c).

For human and animal generation, where point-to-point correspondences i.e. mesh connectivity is fixed, an upsampling technique based on linear layers similar to \cite{lin2021end-to-end} is adopted to obtain a dense mesh with $M$ vertices, ${\bf V} \in \mathbb{R}^{M \times 3} $. Concretely, a coarse mesh with 431 vertices are upsampled to 1723 vertices and then to 6890 vertices using two linear layers as depicted in Fig. \ref{fig:diffsurf_arch} (b). 

For the surface generation of man-made objects, upsampling and refinement based on the improved PointNet++ model \cite{lyu2022conditional} are applied. The input point-normals are mirrored, passed through the UNet-like network based on PointNet subsampling and upsampling layers and finally upsampled by a factor of $\times5$ \cite{slide2023}. The number of points and their feature dimensions processed in the layers are listed in Fig. \ref{fig:diffsurf_arch} (c). Finally, a learning-based surface reconstruction technique called Shape-As-Points (SAP) \cite{Peng2021SAP} is employed to convert the upsampled points ${\bf V} \in \mathbb{R}^{20480 \times 3}$ and normals ${\bf N} \in \mathbb{R}^{20480 \times 3}$ into a mesh.

\section{Appendix: Dataset statistics and details for 3D generation }

We  trained our DiffSurf models separately on publicly available 3D datasets: SURREAL \cite{varol17_surreal}, AMASS \cite{AMASS:2019}, FreiHAND \cite{Freihand2019}, BARC \cite{BARC:2022}, Animal3D \cite{xu2023animal3d} and ShapeNet \cite{chang2015shapenet} pre-processed by  \cite{pointflow}. We follow 3D-CODED \cite{groueix2018b} for the SURREAL train/test split definition. For the ShapeNet object generation, we train a single-class generation model on Airplane, Cabinet, Car, Chair and Lamp. We also train a class-conditioned model using all 13 categories of ShapeNet (Airplane, Bench, Cabinet, Car, Chair, Display, Lamp, Loud speaker, Rifle, Sofa, Table, Telephone, Watercraft). The numbers of mesh instances contained in the training dataset are provided in Table \ref{tab:dataset}. The numbers of vertices in each mesh for respective objects are listed in Table \ref{tab:mesh}. 

To train diffusion transformer efficiently, the training data are down-sampled to coarse-level. For human and animal generation, we used down sampling matrices provided in SMPL \cite{SMPL:2015}, SMAL \cite{Zuffi:CVPR:2017} and MANO \cite{MANO:SIGGRAPHASIA:2017} to do this. Each ShapeNet mesh contains 100,000 points. Thus, we randomly sample 2048 (or 1024) points from them in the dataloader prior to feeding them into the transformer. The body joints are obtained from meshes using joint regressors \cite{SMPL:2015,Zuffi:CVPR:2017} for humans and animals. For ShapeNet objects, we feed sparse latent points generated by SLIDE \cite{slide2023} as body joint tokens to transformer. 

\begin{table}[h]
    \caption{The numbers of meshes contained in the dataset used in training. }
    \centering
    \scalebox{1}{
    \begin{tabular}{cccccc}
    \hline
      AMASS & SURREAL & FreiHAND & BARC & Animal3D & \\
    \hline
    1.2M & 0.23M & 32K & 8K & 3K & \\
    \hline
    \hline
     Airplane & Cabinet & Car & Chair & Lamp & ShapeNet13 \\ 
    \hline
     1000 & 1500 & 5248 & 4746 & 1000 & 30661 \\
    \hline
    \end{tabular}
    }
    \label{tab:dataset}
\end{table}

\begin{table}[h]
    \caption{The numbers of vertices in a mesh for different articulated shapes. }
    \centering
    \begin{tabular}{cccc}
    \hline
     & \#verts & \#verts &  \#Joints \\
     & (Coarse) & (Dense) &  \\
    \hline
    Human body & 431 & 6890 & 14 \\
    Hand & --- & 778 & 21 \\
    Dog &  973 & 3889 & 35\\
    Animal & 973 & 3889 &  35\\
    Airplane & 2048 & 20480 & 16  \\
    Cabinet  & 1024 & 10240 & 16 \\
    Car  & 1024 & 10240 & 16\\
    Chair & 2048 & 20480  & 16  \\
    Lamp  & 2048 & 20480 & 16 \\
    ShapeNet13  & 1024 & 10240 & 0 \\
    \hline
    \end{tabular}
    \label{tab:mesh}
\end{table}

\section{Appendix: Training and implementation details }

The training of DiffSurf involves two steps: training of the diffusion model and the up-sampler are done separately.  We use pre-trained up-sampler models for fixed and varied topology cases. For human generation with fixed connectivity, we trained an upsampling network similar to METRO by giving synthetic images (shaded images rendered without texture) of SURREAL human body meshes facing front as input to the network and using the same losses used in  \cite{lin2021end-to-end}. Then, only upsampler is extracted from the whole network model. This process could possibly be simplified by removing the image encoder and transformer encoder from METRO and feeding coarse meshes directly as input to the upsampler during training.  For animal cases, we used a sparse upsampler model provided by \cite{Zuffi:CVPR:2017}.  For topologically varying man made objects, we used the pre-trained models of  up-samplers and SAP models made available  by the authors of SLIDE \cite{slide2023}. Specifically, we tested the "normal$\_$symmetry" and "normal$\_$symmetry$\_$noise$\_0.02$" models for our surface reconstruction.   

Our diffusion transformer model is trained with a batch size of 256 for 400 epochs on 4 NVIDIA V100 GPUs for the SURREAL dataset, and for 200 epochs on 8 NVIDIA A100 GPUs for the AMASS dataset. It takes about 1 day for both cases. For the BARC, Animal3D and ShapeNet objects, we extend the training of diffusion transformer to 4000-8000 epochs because they contain fewer meshes than SURREAL and AMASS. The up-sampler of human generation is trained for 50 epochs. We use the Adam optimizer for training our models, while reducing the learning rate by a factor of 10 after $1/2$ of the total training epochs beginning from $1 \times 10^{-4}$. For the training objective of DiffSurf, we adopt the v-prediction parameterization \cite{salimans2022progressive,lucidrain}. We employ the DDIM \cite{song2020denoising} sampler along with a sigmoid variance scheduler. The diffusion time step is set to $T =1000$ and sampling steps in the range [1-250] are tested. 

We implemented our models in Pytorch. Our implementation is based on METRO \cite{lin2021end-to-end} and U-ViT \cite{bao2022all}. We will make our code publicly available.

\section{Appendix: Impact of training dataset size in human generation}

Figure  \ref{fig:dataset_scale} visualizes mesh generation results of DiffSurf trained with different numbers of training meshes (2.3K, 23K and 230K) from SURREAL. Training epochs are 8000, 2000 and 400, respectively. Note that the results compared are sampled from the same random noise seeds. With 2.3K training meshes, some of generated results exhibit unnatural bending of joints and shrinkage of hands. Adding more training meshes mitigates these issues.

\begin{figure*}[t]
\begin{center}
 \includegraphics[width=\linewidth]{images/supplemental/dataset_scale.png}
 \caption{Visualizations of unconditional mesh generation results using the models trained on SURREAL but varying the training dataset size. DiffSurf is trained on  2.3K, 23K and 230K SURREAL meshes.  }
 \label{fig:dataset_scale}
\end{center}
\end{figure*}

\section{Appendix: The impact of the guidance scale in classifier free guidance}

DiffSurf can generate a mesh that is conditioned on 3D skeleton landmark locations, such as those obtained using motion capture and image-based 3D pose regressors. Essentially, this process of conditional mesh generation involves feeding 3D body joint locations as tokens into the diffusion transformer and setting the timestep to $t_y=0$. Naively feeding 3D joint locations into DiffSurf results in slight discrepancies between the mesh and the joints. To address this, we leverage CFG to push the mesh toward joint locations and improve alignments between them  (Fig. \ref{fig:cfg}). We found that setting the CFG weight to around $s_{\rm g} = 1$ effectively improves alignment while preserving the mesh structure. Excessively increased CFG weights, e.g., $s_{\rm g} > 3$, can result in distortion of the mesh. 

\begin{figure*}[t]
\begin{center}
 \includegraphics[width=0.7\linewidth]{images/supplemental/method_flow.png}
 \caption{Visualizations of meshes by varying the guidance scale of classifier free guidance (CFG).  Increasing the CFG scaling weight $s_{\rm g}$ helps push a mesh toward 3D joint locations when performing pose conditional generation. In our experiments, by setting $s_{\rm g}$ to around 0.5-1, the alignment between the mesh and joint conditions is enhanced, while preserving mesh structure. Using excessively high CFG weights can result in distorting a mesh, e.g. $s_{\rm g} > 3$.  }
 \label{fig:cfg}
\end{center}
\end{figure*}

\section{Appendix: Details on the loss terms in control point deformation }  In below, we describe each loss term used in control point deformation. Let ${\bf v} \in \mathbb{R}^{N \times 3}$, ${\bf e} \in \mathbb{R}^{E \times 1}$ and ${\bf \delta} \in \mathbb{R}^{N \times 3}$ be the current predictions for 3D coordinates, edge lengths and Laplacian coordinates of coarse mesh, respectively. Letting also ${\bf v}_{\rm SDS} \in \mathbb{R}^{N \times 3}$, ${\bf e}_{\rm SDS} \in \mathbb{R}^{E \times 1}$ and ${\bf \delta}_{\rm SDS} \in \mathbb{R}^{N \times 3}$ denote the SDS targets for 3D coordinates, edge lengths and Laplacian coordinates of coarse mesh, respectively. The 3D coordinates of SDS target are obtained by ${\bf v}_{\rm SDS} = {\bf v} - {\bf grad}_{\rm SDS}^{\rm v}$ where ${\bf grad}_{\rm SDS}^{\rm v}$ is the vertex components of the SDS gradients. Then, the losses $L_{\rm SDS}$, $L_{\rm SDS}^{\rm edge}$ and  $L_{\rm SDS}^{\rm lap}$ are defined by the distances between the optimized variables and the SDS targets:
\begin{align}
\nonumber &L_{\rm SDS} =  ||{\bf v} -  {\bf v}_{\rm SDS}||_2^2/N  \\ \nonumber
\nonumber &L_{\rm SDS}^{\rm edge} =  ||{\bf e} -  {\bf e}_{\rm SDS}||_2 ^2/E\\ \nonumber
\nonumber &L_{\rm SDS}^{\rm lap} =  ||{\bf \delta} -  {\bf \delta}_{\rm SDS}||_2^2 /N \\ \nonumber
\end{align}

$L_{\rm consist}$ maintains the consistency between the joint and mesh prediction, defined by the distances between the optimized joints ${\bf j} \in \mathbb{R}^{J \times 3}$ and the regressed joints ${\bf j}_{\rm reg} \in \mathbb{R}^{J \times 3}$. The regressed joints ${\bf j}_{\rm reg}$ are calculated from the mesh vertices using the joint regressor, ${\bf j}_{\rm reg} = \cal{J}{\bf V}$, where $\cal{J}$ is a joint regressor matrix and ${\bf V}$ is the vertex coordinates of a dense mesh. Then $L_{\rm consist}$ is defined as follows:
\begin{align}
\nonumber L_{\rm consist} =  ||{\bf j} -  {\bf j}_{\rm reg}||_2^2/J  \\ \nonumber
\end{align}

$L_{\rm CP}$ quantifies the distances between the optimized joint locations and the control points. 
\begin{align}
\nonumber L_{\rm CP} =  ||{\bf j}_{\rm CP} -  \bar{\bf j}_{\rm CP}||_2^2 / J_{\rm CP}  \\ \nonumber
\end{align}
where ${\bf j}_{\rm CP} \in \mathbb{R}^{J_{\rm CP} \times 3}$ and $\bar{\bf j}_{\rm CP} \in \mathbb{R}^{J_{\rm CP} \times 3}$ are the optimized and the specified control points, respectively. 

%Figure \ref{fig:cp_loss} shows the comparisons of the loss terms. Using $L_{\rm SDS}$ and $L_{\rm CP}$, DiffSurf is able to fit a human mesh toward control points but there remains some distances between them. Incorporating $L_{\rm consist}$ improves the fit but introduces distortions around the control points. Adding $L_{\rm SDS}^{\rm edge}$ and $L_{\rm SDS}^{\rm lap}$ remedies this issue by considering differential properties of the coarse mesh to preserve its local geometry.   

\section{Appendix: Network architecture for human mesh recovery }

%The network architecture of the 3D pose regressor is similar to METRO \cite{lin2021end-to-end} but it only regresses 14 body joint locations. The 3D pose regressor consists of transformer blocks with ten layers. Each block has the hidden layer with 256 channels. We employ HRNet-w48 \cite{sun2019deep} ($256 \times 192$ input image resolution) as its CNNs backbone, initialized with weights pre-trained on COCO dataset. The weights in the transformer decoder are randomly initialized.  

The overall architecture of our human mesh recovery model based on DiffSurf is depicted in Fig. \ref{fig:hnr_arch}. It integrates an image-based 3D pose regressor with DiffSurf to achieve human mesh recovery. The network architecture of our 3D pose regressor is illustrated in Fig. \ref{fig:hnr_arch} left. This can be thought of as a variant of Mesh Transformer \cite{lin2021end-to-end}, which is modified to output a 3D pose solely.  The 3D pose regressor consists of transformer blocks with ten layers. Each block has the hidden layer with 256 channels. We employ HRNet-w48 \cite{sun2019deep} ($256 \times 192$ input image resolution) as its CNNs backbone, initialized with weights pre-trained on COCO dataset. Grid features corresponding to an $8\times6$ feature map output from HRNet-w48 are input to transformer directly as tokens along with the learned position embedding summed on them. In addition, these image features are passed through a convolution layer and then fed into the transformer as body joint tokens. Once the 3D pose is predicted by the 3D pose regressor, conditional mesh generation is performed by inputting the predicted 3D body joint locations as queries to DiffSurf and set their corresponding timesteps to $t_y=0$. Finally, a dense mesh is obtained by upsampler from a coarse mesh generated by DiffSurf.

%It consists of 1) a diffusion transformer and 2) a mesh upsampler (Fig \ref{fig:overview}). 

%The inputs to the diffusion transformer consist of noisy  3D coordinates for a set of joint query tokens $Q_{\rm J}=\{ Q^1_{\rm J} \ldots Q^J_{\rm J} \} $ and coarse vertex query tokens $Q_{\rm V}= \{ Q^1_{\rm V} \ldots Q^N_{\rm V} \} $, corresponding to an articulated body mesh comprising $J$ joints and $N$ vertices. The diffusion transformer processes these two modalities of data and their corresponding timesteps as tokens. Our diffusion transformer consists of transformer blocks with five  layers. These blocks have the hidden layers with the dimension of 256 channels. The input and output MLPs convert between 3-dimensional noisy 3D coordinates/noise prediction and 256 dimensional transformer embedding features.

% timesteps
% parameters?

\begin{figure*}[t]
\begin{center}
 \includegraphics[width=\linewidth]{images/supplemental/hmr_architecture.png}
 \caption{The network architecture of human mesh recovery model. }
 \label{fig:hnr_arch}
\end{center}
\end{figure*}

\section{Appendix: Human mesh recovery results with multiple hypotheses } 

Human mesh recovery based on DiffSurf is comparable to previous human mesh recovery techniques. However, since DiffSurf does not explicitly relate its generation to an image, performance is affected by random input mesh noise ${\bf x}_T$ that alters body styles and twisting joint angles of generations. Here, we show how multiple hypotheses on the input mesh noise can possibly improve DiffSurf's performance further. Similar to the idea presented in the recent model-based human mesh recovery work \cite{cho2023generative}, where the multiple hypotheses on the pose generated by diffusion models are leveraged to produce mesh recovery results, we generated mesh recovery results from multiple hypotheses of mesh noise inputs. With 20 hypotheses, DiffSurf is competitive with PARE \cite{Kocabas_PARE_2021} on 3DPW and HMDiff \cite{dat2023} on Human3.6M. Note that the results shown on Table \ref{tab:multiple_hypothesis} relies on the GT 3D poses for selecting the minimum error hypothesis. While this approach has been a common practice \cite{li2019, Jahangiri2017} in the multi-hypothesis 3D human pose estimation, we acknowledge that it only provides upper bounds of estimation and does not conduct a fair comparison. Nonetheless these results indicate that the use of multiple hypotheses is a promising direction for further performance improvements. Future work could explore an aggregation technique \cite{shan2023diffusion} from  multiple hypotheses of meshes from DiffSurf based on e.g. input 3D poses or other 2D evidences. 

%\subsection{Qualitative results} 
\begin{table}[t]
%\captionsetup[subtable]{justification=centering}
\centering
%\begin{subtable}[t]{.53\linewidth}
\caption{Comparisons with 3D mesh recovery approaches on 3DPW. No fine-tuning on 3DPW performed. }
    \scalebox{0.9}[0.9]{
\begin{tabular}{c c c c c c}
\hline 
 \multirow{2}{*}{Method} & \multicolumn{2}{c}{3DPW} & \multicolumn{2}{c}{Human 3.6M}\\
  &  MPVE $\downarrow$ &  PA-MPJPE $\downarrow$ & MPJPE $\downarrow$ &  PA-MPJPE $\downarrow$ \\
\hline  
 METRO \cite{lin2021end-to-end} & 119.1 & 63.0 & 54.0 & 36.7 \\
 PARE \cite{Kocabas_PARE_2021} & {\bf 97.9} & 50.9 & 76.8 & 50.6 \\   
 HMDiff \cite{dat2023} & --- & ---  & 49.3 & {\bf 32.4} \\
 DiffHMR (n=1) \cite{luo2021diffusion} & 114.6 & 58.5 & --- & --- \\
 DiffHMR (n=10) \cite{luo2021diffusion} & 110.9 & 56.5  & --- & --- \\
 DiffHMR (n=20) \cite{luo2021diffusion} & 109.8 & 55.9  & --- & -- \\
 DiffSurf (n=1) &  108.0 & 53.7  & 48.9 & 36.1 \\
 DiffSurf (n=10)  & 100.2  & 49.9  & 46.9 & 34.5 \\  
DiffSurf (n=20)  & \underline{98.5}   & {\bf  49.1} & {\bf 46.4} & \underline{33.9} \\   
\hline 
\end{tabular}
\label{tab:multiple_hypothesis}
}
\end{table}

%\section{Appendix: Performance with other 3D pose regressors }

\section{Appendix: Qualitative comparison against Mesh Transformer (METRO)}

Figure \ref{fig:vs_metro} qualitatively compares our results against  Mesh transformer (METRO) \cite{lin2021end-to-end}. It is known that METRO produces results with noise especially on images that are not visually close to training set. Also, METRO tends to distort a mesh on some images as it is based on a model-free mesh regressor and does not strongly constrain the mesh output to the pre-defined body shape subspace. On the other hand, DiffSurf generates a smoother and less distorted mesh through a diffusion process from 3D pose conditions. Since DiffSurf does not directly relate its mesh generation to an image, currently it lacks the ability to model subtle effects like face orientations which needs to be inferred from image evidences.  

\section{Appendix: Qualitative comparison between with and w/o SDS fitting}

Our fitting approach improves mesh alignment toward 2D keypoint locations, e.g. around hands and feet, by incorporating priors derived  from DiffSurf based on the SDS loss (Fig. \ref{fig:fitting}).

\section{Appendix: Qualitative results on 3D mesh processing tasks}

 In Figs. \ref{fig:car} and \ref{fig:more_interpolation2}, we show unconditional generation result (Car and Cabinet) and shape morphing results of Chair, respectively. Figures \ref{fig:more_human}, \ref{fig:more_hand } and \ref{fig:more_animal} visualizes additional qualitative results of unconditional 3D mesh generations on humans, hands and animals, respectively. In Figs. \ref{fig:more_body_shape}, \ref{fig:more_interpolation1}, and \ref{fig:more_refinement}, we provide examples of 3D human mesh processing such as body shape variation, shape interpolation, mesh refinement and control point deformation, respectively.

\begin{figure*}[t]
\begin{center}
 \includegraphics[width=\linewidth]{images/supplemental/vs_metro.png}
 \caption{Qualitative comparison against Mesh Transformer (METRO) \cite{lin2021end-to-end}. }
 \label{fig:vs_metro}
\end{center}
\end{figure*}

\begin{figure*}[t]
\begin{center}
 \includegraphics[width=\linewidth]{images/supplemental/fitting.png}
 \caption{Qualitative comparison between DiffSurf results with and w/o SDS fitting. }
 \label{fig:fitting}
\end{center}
\end{figure*}

\begin{figure*}[t]
\begin{center}
 \includegraphics[width=\linewidth]{images/supplemental/car_cabinet.png}
 \caption{Class-level unconditional generation results of Car and Cabinet.  }
 \label{fig:car}
\end{center}
\end{figure*}

\begin{figure*}[t]
\begin{center}
 \includegraphics[width=1\linewidth]{images/supplemental/interpolation_chair.png}
 \caption{Chair shape morphing results. }
 \label{fig:more_interpolation2}
\end{center}
\end{figure*}

\begin{figure*}[t]
\begin{center}
 \includegraphics[width=\linewidth]{images/supplemental/human_mesh_generation.png}
 \caption{Human mesh generation results. }
 \label{fig:more_human}
\end{center}
\end{figure*}

\begin{figure*}[t]
\begin{center}
 \includegraphics[width=\linewidth]{images/supplemental/hand_mesh_generation.png}
 \caption{Hand mesh generation results. }
 \label{fig:more_hand }
\end{center}
\end{figure*}

\begin{figure*}[t]
\begin{center}
 \includegraphics[width=\linewidth]{images/supplemental/anima_mesh_generation.png}
 \caption{Animal mesh generation results. }
 \label{fig:more_animal}
\end{center}
\end{figure*}

\begin{figure*}[t]
\begin{center}
 \includegraphics[width=1\linewidth]{images/supplemental/body_shape_variation.png}
 
 \caption{Body shape variation. Top: Single step approach. Feeding 3D joint locations into DiffSurf as conditions and performing sampling by varying random noise,  we are able to generate meshes in different body shapes. However, this approach does not allow for the changes in body heights and segment lengths.  Bottom: Two-step approach. The first step performs unimodal generation to create a batch of skeletons with different body poses and styles and then adjusts the segment lengths of one of generated skeletons based on others in the batch. Inputting these modified skeletons into DiffSurf and performing pose conditional mesh generation, we can generate meshes in diverse body styles while maintaining the pose. }
 \label{fig:more_body_shape}
\end{center}
\end{figure*}

\begin{figure*}[t]
\begin{center}
 \includegraphics[width=0.85\linewidth]{images/supplemental/interpolation.png}
 \caption{Human shape and pose morphing results. }
 \label{fig:more_interpolation1}
\end{center}
\end{figure*}

\begin{figure*}[t]
\begin{center}
 \includegraphics[width=\linewidth]{images/supplemental/refinement.png}
 \caption{Sequence of meshes constructed during shape refinement process. }
 \label{fig:more_refinement}
\end{center}
\end{figure*}

%\begin{figure*}[t]
%\begin{center}
% \includegraphics[width=\linewidth]{images/supplemental/control_points.png}
% \caption{Control point deformation with five control points (Wrists, ankles and head).  }
% \label{fig:more_control_points}
%\end{center}
%\end{figure*}

\section{Appendix: Qualitative results on 3D mesh recovery }

Figure \ref{fig:more_hmr} shows additional human mesh recovery results of DiffSurf where a 3D human mesh is predicted from a single image.

\begin{figure*}[t]
\begin{center}
 \includegraphics[width=\linewidth]{images/supplemental/hmr_qualitative.png}
 \caption{Visualization of human mesh recovery results.}
 \label{fig:more_hmr}
\end{center}
\end{figure*}

%\bibliographystyle{splncs04}
%\bibliography{main}

%\end{document}
