# Supplementary material for: DiffSurf: A Transformer-based Diffusion Model for Generating and Reconstructing 3D Surfaces in Pose
Source: arXiv:2408.14860 source file (2024-08-27)
Supplement: Supplementary file 2 [file X_suppl.tex]

\section{Appendix: Implementation}

We implemented our models in Pytorch. Our implementation is based on METRO \cite{lin2021end-to-end} and U-ViT \cite{bao2022all}. We are planning to make our code publicly available upon acceptance. 

\section{Appendix: Dataset statistics }

The numbers of mesh instances contained in the training dataset are provided in Table \ref{tab:dataset} and the numbers of vertices in a mesh for respective articulated shapes are listed in Table \ref{tab:mesh}. To train diffusion transformer efficiently, the training meshes are down-sampled to coarser meshes with less than 1K vertices using down sampling matrices provided in SMPL \cite{SMPL:2015}, SMAL \cite{Zuffi:CVPR:2017} and MANO \cite{MANO:SIGGRAPHASIA:2017}. The body joints are obtained using joint regressor matrices that are also provided by these models. 

\begin{table}[h]
    \caption{The numbers of meshes contained in the dataset used in training. }
    \centering
    \scalebox{0.9}{
    \begin{tabular}{ccccc}
    \hline
      AMASS & SURREAL & FreiHAND & BARC & Animal3D  \\
    \hline
    1.2M & 0.23M & 32K & 8K & 3K \\
    \hline
    \end{tabular}
    }
    \label{tab:dataset}
\end{table}

\begin{table}[h]
    \caption{The numbers of vertices in a mesh for different articulated shapes. }
    \centering
    \begin{tabular}{ccccc}
    \hline
     & \#verts & \#verts & \#verts & \#Joints \\
     & (level0) & (level1) & (level2) &  \\
    \hline
    Human body & 6890 & 1723 & 431 & 14 \\
    Hand & 778 & --- & --- & 21 \\
    Dog & 3889 & 973 & --- & 35\\
    Animal & 3889 & 973 & --- &  35\\
    Airplane & 2048 &--- & --- & 16  \\
    Chair  & 2048 & --- & --- & 0\\
    Lamp  & 2048 & --- & --- & 16\\
    \hline
    \end{tabular}
    \label{tab:mesh}
\end{table}

\section{Appendix: Impact of training dataset size }

Figure  \ref{fig:dataset_scale} visualizes mesh generation results of Mesh Diffuser trained with different numbers of training meshes (2.3K, 23K and 230K) from SURREAL. Training epochs are 8000, 2000 and 400, respectively. Note that the results compared are sampled from the same random noise seeds. With 2.3K training meshes, some of generated results exhibit unnatural bending of joints and shrinkage of hands. Adding more training meshes mitigates these issues.

\begin{figure*}[t]
\begin{center}
 \includegraphics[width=\linewidth]{images/supplemental/dataset_scale.png}
 \caption{Visualizations of unconditional mesh generation results using the models trained on SURREAL but varying the training dataset size. Mesh Diffuser is trained on  2.3K, 23K and 230K SURREAL meshes.  }
 \label{fig:dataset_scale}
\end{center}
\end{figure*}

\section{Appendix: Network architecture for human mesh recovery }

%The network architecture of the 3D pose regressor is similar to METRO \cite{lin2021end-to-end} but it only regresses 14 body joint locations. The 3D pose regressor consists of transformer blocks with ten layers. Each block has the hidden layer with 256 channels. We employ HRNet-w48 \cite{sun2019deep} ($256 \times 192$ input image resolution) as its CNNs backbone, initialized with weights pre-trained on COCO dataset. The weights in the transformer decoder are randomly initialized.  

The overall architecture of our human mesh recovery model based on Mesh Diffuser is depicted in Fig. \ref{fig:hnr_arch}. It integrates an image-based 3D pose regressor with Mesh Diffuser to achieve human mesh recovery. The network architecture of our 3D pose regressor is illustrated in Fig. \ref{fig:hnr_arch} left. This can be thought of as a variant of Mesh Transformer \cite{lin2021end-to-end} and Mesh Graphormer \cite{lin2021-mesh-graphormer}, which is modified to output a 3D pose solely.  The 3D pose regressor consists of transformer blocks with ten layers. Each block has the hidden layer with 256 channels. We employ HRNet-w48 \cite{sun2019deep} ($256 \times 192$ input image resolution) as its CNNs backbone, initialized with weights pre-trained on COCO dataset. Grid features corresponding to an $8\times6$ feature map output from HRNet-w48 are input to transformer directly as tokens along with the learned position embedding summed on them. In addition, these image features are passed through a convolution layer and then fed into the transformer as body joint tokens. Once the 3D pose is predicted by the 3D pose regressor, conditional mesh generation is performed by inputting the predicted 3D body joint locations as queries to Mesh Diffuser and set their corresponding timesteps to $t_y=0$. Finally, a dense mesh is obtained by upsampler from a coarse mesh generated by Mesh Diffuser.

%It consists of 1) a diffusion transformer and 2) a mesh upsampler (Fig \ref{fig:overview}). 

%The inputs to the diffusion transformer consist of noisy  3D coordinates for a set of joint query tokens $Q_{\rm J}=\{ Q^1_{\rm J} \ldots Q^J_{\rm J} \} $ and coarse vertex query tokens $Q_{\rm V}= \{ Q^1_{\rm V} \ldots Q^N_{\rm V} \} $, corresponding to an articulated body mesh comprising $J$ joints and $N$ vertices. The diffusion transformer processes these two modalities of data and their corresponding timesteps as tokens. Our diffusion transformer consists of transformer blocks with five  layers. These blocks have the hidden layers with the dimension of 256 channels. The input and output MLPs convert between 3-dimensional noisy 3D coordinates/noise prediction and 256 dimensional transformer embedding features.

% timesteps
% parameters?

\begin{figure*}[t]
\begin{center}
 \includegraphics[width=\linewidth]{images/supplemental/hmr_architecture.png}
 \caption{The network architecture of human mesh recovery model. }
 \label{fig:hnr_arch}
\end{center}
\end{figure*}

\section{Appendix: Ablation study on network components }

To conduct the ablation study on our diffusion transformer model's components, we modified  the elements in it and compared performances. The basic network architecture that we originate the ablation study from is an adaptation of U-ViT \cite{bao2022all}, tailored to handle 3D mesh and body joint tokens (Table \ref{tab:ablation} top row). We investigated the impacts of long skip connections, different methods of incorporating time embedding, position embedding constructions and the effect of varying the network layer types (transformer or MLPs). As shown in Table \ref{tab:ablation}, the switch in the layer type from transformer to MLPs yields the most significant impact, indicating the most critical component of Mesh Diffuser is the transformer layer. As opposed to U-ViT \cite{bao2022all} for image generation, the use of long skip connection does not contribute to improving 3D human mesh generation. This may be attributed to the current form of the diffusion transformer in Mesh Diffuser primarily processing coarse-level mesh vertices. Expressive human body generation that incorporates fine-grained details like finger pose changes and facial expressions could potentially benefit from long-skip connections.   

\begin{table}[h]
%\captionsetup[subtable]{justification=centering}
\centering
%\begin{subtable}[t]{.53\linewidth}
\caption{Ablation study on network components. }
\scalebox{0.85}[0.85]{
\begin{tabular}{c c c c c}
\hline 
Base & Pos emb & Time emb & Long skip & 1NNA $\downarrow$ \\
\hline 
Transformer &  Learned & Token & Yes & 55.6  \\
Transformer &  Learned & Token & {\bf No} & {\bf 54.4} \\
Transformer & Learned & {\bf Add} & Yes & 55.4  \\
Transformer &  {\bf 3D Template} & Token & Yes & 54.8 \\
{\bf MLP} &  Learned & Token & Yes & 92.6  \\
\hline 
\end{tabular}
\label{tab:ablation}
}
\end{table}

\begin{comment}

\section{Rationale}
\label{sec:rationale}
% 
Having the supplementary compiled together with the main paper means that:
% 
\begin{itemize}
\item The supplementary can back-reference sections of the main paper, for example, we can refer to \cref{sec:intro};
\item The main paper can forward reference sub-sections within the supplementary explicitly (e.g. referring to a particular experiment); 
\item When submitted to arXiv, the supplementary will already included at the end of the paper.
\end{itemize}
% 
To split the supplementary pages from the main paper, you can use \href{https://support.apple.com/en-ca/guide/preview/prvw11793/mac#:~:text=Delete%20a%20page%20from%20a,or%20choose%20Edit%20%3E%20Delete).}{Preview (on macOS)}, \href{https://www.adobe.com/acrobat/how-to/delete-pages-from-pdf.html#:~:text=Choose%20%E2%80%9CTools%E2%80%9D%20%3E%20%E2%80%9COrganize,or%20pages%20from%20the%20file.}{Adobe Acrobat} (on all OSs), as well as \href{https://superuser.com/questions/517986/is-it-possible-to-delete-some-pages-of-a-pdf-document}{command line tools}.

\end{comment}

%\section{Appendix: More quantitative evaluation with other metrics  }

\section{Appendix: Human mesh recovery results with multiple hypotheses } 

As shown in Table \ref{tab:SOTA}, Mesh Diffuser is comparable to previous human mesh recovery techniques. However, since Mesh Diffuser does not explicitly relate its generation to an image, performance is affected by random input mesh noise ${\bf x}_T$ that alters body styles of generations. Here, we show how multiple hypotheses on the input mesh noise can possibly improve Mesh Diffuser's performance further. Similar to the idea presented in the recent parametric human mesh recovery work \cite{cho2023generative}, where the multiple hypotheses on the pose generated by diffusion models are leveraged to produce mesh recovery results, we generated mesh recovery results from multiple hypotheses of mesh noise inputs. With 20 hypotheses, Mesh Diffuser is competitive with PARE \cite{Kocabas_PARE_2021} on 3DPW and HMDiff \cite{dat2023} on Human3.6M. Note that the results shown on Table \ref{tab:multiple_hypothesis} relies on the GT 3D poses for selecting the minimum error hypothesis. While this approach has been a common practice \cite{li2019, Jahangiri2017} in the multi-hypothesis 3D human pose estimation, we acknowledge that it only provides upper bounds of estimation and does not conduct a fair comparison. Nonetheless these results indicate that the use of multiple hypotheses is a promising direction for further performance improvements. Future work could explore an aggregation technique \cite{shan2023diffusion} from  multiple hypotheses of meshes from Mesh Diffuser based on e.g. input 3D poses or other 2D evidences. 

%\subsection{Qualitative results} 
\begin{table}[t]
%\captionsetup[subtable]{justification=centering}
\centering
%\begin{subtable}[t]{.53\linewidth}
\caption{Comparisons with 3D mesh recovery approaches on 3DPW. No fine-tuning on 3DPW performed. }
    \scalebox{0.8}[0.8]{
\begin{tabular}{c c c c c c}
\hline 
 \multirow{2}{*}{Method} & \multicolumn{2}{c}{3DPW} & \multicolumn{2}{c}{Human 3.6M}\\
  & \hspace{-10pt} MPVE $\downarrow$ &\hspace{-10pt}  PA-MPJPE $\downarrow$ & \hspace{-10pt} MPJPE $\downarrow$ & \hspace{-10pt} PA-MPJPE $\downarrow$ \\
\hline  
 METRO \cite{lin2021end-to-end} & 119.1 & 63.0 & 54.0 & 36.7 \\
 PARE \cite{Kocabas_PARE_2021} & {\bf 97.9} & 50.9 & 76.8 & 50.6 \\   
 HMDiff \cite{dat2023} & --- & ---  & 49.3 & {\bf 32.4} \\
 DiffHMR (n=1) \cite{luo2021diffusion} & 114.6 & 58.5 & --- & --- \\
 DiffHMR (n=10) \cite{luo2021diffusion} & 110.9 & 56.5  & --- & --- \\
 DiffHMR (n=20) \cite{luo2021diffusion} & 109.8 & 55.9  & --- & -- \\
 MeshDiffuser (n=1) &  108.0 & 53.7  & 48.9 & 36.1 \\
 MeshDiffuser (n=10)  & 100.2  & 49.9  & 46.9 & 34.5 \\  
MeshDiffuser (n=20)  & \underline{98.5}   & {\bf  49.1} & {\bf 46.4} & \underline{33.9} \\   
\hline 
\end{tabular}
\label{tab:multiple_hypothesis}
}
\end{table}

%\section{Appendix: Performance with other 3D pose regressors }

\section{Appendix: Details on the loss terms in control point deformation } Equation (\ref{eq:deform}) defines the total loss $L_{\rm def}$ for control point deformation. In below, we describe each loss term. Let ${\bf v} \in \mathbb{R}^{N \times 3}$, ${\bf e} \in \mathbb{R}^{E \times 1}$ and ${\bf \delta} \in \mathbb{R}^{N \times 3}$ be the current predictions for 3D coordinates, edge lengths and Laplacian coordinates of coarse mesh, respectively. Letting also ${\bf v}_{\rm SDS} \in \mathbb{R}^{N \times 3}$, ${\bf e}_{\rm SDS} \in \mathbb{R}^{E \times 1}$ and ${\bf \delta}_{\rm SDS} \in \mathbb{R}^{N \times 3}$ denote the SDS targets for 3D coordinates, edge lengths and Laplacian coordinates of coarse mesh, respectively. The 3D coordinates of SDS target are obtained by ${\bf v}_{\rm SDS} = {\bf v} - {\bf grad}_{\rm SDS}^{\rm v}$ where ${\bf grad}_{\rm SDS}^{\rm v}$ is the vertex components of the SDS gradients defined in Eq. \ref{eq:SDS}. Then, the SDS targets of edge and Laplacian arn, ${\bf e}_{\rm SDS}$ and ${\bf \delta}_{\rm SDS}$, are obtained from  ${\bf v}_{\rm SDS}$ using know mesh connectivity. Consequently, the losses $L_{\rm SDS}$, $L_{\rm SDS}^{\rm edge}$ and  $L_{\rm SDS}^{\rm lap}$ are defined by the distances between the optimized variables and the SDS targets:
\begin{align}
\nonumber &L_{\rm SDS} =  ||{\bf v} -  {\bf v}_{\rm SDS}||_2^2/N  \\ \nonumber
\nonumber &L_{\rm SDS}^{\rm edge} =  ||{\bf e} -  {\bf e}_{\rm SDS}||_2 ^2/E\\ \nonumber
\nonumber &L_{\rm SDS}^{\rm lap} =  ||{\bf \delta} -  {\bf \delta}_{\rm SDS}||_2^2 /N \\ \nonumber
\end{align}

$L_{\rm consist}$ maintains the consistency between the joint and mesh prediction, defined by the distances between the optimized joints ${\bf j} \in \mathbb{R}^{J \times 3}$ and the regressed joints ${\bf j}_{\rm reg} \in \mathbb{R}^{J \times 3}$. The regressed joints ${\bf j}_{\rm reg}$ are calculated from the mesh vertices using the joint regressor, ${\bf j}_{\rm reg} = \cal{J}{\bf V}$, where $\cal{J}$ is a joint regressor matrix and ${\bf V}$ is the vertex coordinates of a dense mesh. Then $L_{\rm consist}$ is defined as follows:
\begin{align}
\nonumber L_{\rm consist} =  ||{\bf j} -  {\bf j}_{\rm reg}||_2^2/J  \\ \nonumber
\end{align}

$L_{\rm CP}$ quantifies the distances between the optimized joint locations and the control points. 
\begin{align}
\nonumber L_{\rm CP} =  ||{\bf j}_{\rm CP} -  \bar{\bf j}_{\rm CP}||_2^2 / J_{\rm CP}  \\ \nonumber
\end{align}
where ${\bf j}_{\rm CP} \in \mathbb{R}^{J_{\rm CP} \times 3}$ and $\bar{\bf j}_{\rm CP} \in \mathbb{R}^{J_{\rm CP} \times 3}$ are the optimized and the specified control points, respectively. 

Figure \ref{fig:cp_loss} shows the comparisons of the loss terms. Using $L_{\rm SDS}$ and $L_{\rm CP}$, Mesh Diffuser is able to fit a human mesh toward control points but there remains some distances between them. Incorporating $L_{\rm consist}$ improves the fit but introduces distortions around the control points. Adding $L_{\rm SDS}^{\rm edge}$ and $L_{\rm SDS}^{\rm lap}$ remedies this issue by considering differential properties of the coarse mesh to preserve its local geometry.   

\begin{figure*}[t]
\begin{center}
 \includegraphics[width=\linewidth]{images/supplemental/cp_losses.png}
 \caption{Comparisons on control point deformation losses.  }
 \label{fig:cp_loss}
\end{center}
\end{figure*}

\section{Appendix: Qualitative comparison against Mesh Transformer (METRO)}

Figure \ref{fig:vs_metro} qualitatively compares our results against  Mesh transformer (METRO) \cite{lin2021end-to-end}. It is known that METRO produces results with noise especially on images that are not visually close to training set. Also, METRO tends to distort a mesh on some images as it is based on a vertex-based mesh regressor and does not strongly constrain the mesh output to the pre-defined body shape subspace. On the other hand, Mesh Diffuser generates a smoother and less distorted mesh through a diffusion process from 3D pose conditions. Since Mesh Diffuser does not directly relate its mesh generation to an image, currently it lacks the ability to model subtle effects like face orientations which needs to be inferred from image evidences.  

\section{Appendix: Limitations }

While Mesh Diffuser implicitly considers body shapes and poses as distinct variables by introducing mesh and body joint tokens and treating them as distinct modalities, it does not explicitly establish disentangle representation of body shape and pose. Thus, occasionally we found that the body shape changes when he pose changes during pose-conditional mesh generation. Likewise, male/female is not consistent across all frames during body shape variation, as it can be seen from Fig. \ref{fig:more_body_shape}. A  method for establishing disentangled representation of body shape/pose and controlling a body model based on attributes would be a useful tool in applications that require precise controls over body shape and pose.  

With 230K training meshes, MeshDiffuser very rarely generates meshes that exhibit  artifacts on extreme poses (Fig. \ref{fig:failures} top)  but more cases are found in less data settings (supplemental Fig. 10). Self-intersections of the body parts occur occasionally. Currently, like most of other 3D generative models, our method is limited to category-level generation, except on Animal3D dataset (40 species).%, where its categorical diversity determined by the dataset trained on.  

\begin{figure}[t]
\begin{center}
 \includegraphics[width=0.5\linewidth]{images/rebutttal/failure.png}
 \caption{Failure cases. }
 \label{fig:failures}
\end{center}
\end{figure}

\section{Appendix: More qualitative results on 3D mesh processing tasks}

Figures \ref{fig:more_human}, \ref{fig:more_hand } and \ref{fig:more_animal} visualizes additional qualitative results of unconditional 3D mesh generations on humans, hands and animals, respectively. In Figs. \ref{fig:more_body_shape}, \ref{fig:more_interpolation}, \ref{fig:more_refinement} and \ref{fig:more_control_points}, we provide more examples of body shape variation, shape interpolation, mesh refinement and control point deformation, respectively.

\begin{figure*}[t]
\begin{center}
 \includegraphics[width=\linewidth]{images/supplemental/vs_metro.png}
 \caption{Qualitative comparison against Mesh Transformer (METRO) \cite{lin2021end-to-end}. }
 \label{fig:vs_metro}
\end{center}
\end{figure*}

\section{Appendix: Qualitative comparison between with and w/o SDS fitting}

Our fitting approach improves mesh alignment toward 2D keypoint locations, e.g. around hands and feet, by incorporating priors derived  from Mesh Diffuser based on the SDS loss (Fig. \ref{fig:fitting}). 

\begin{figure*}[t]
\begin{center}
 \includegraphics[width=\linewidth]{images/supplemental/fitting.png}
 \caption{Qualitative comparison between Mesh Diffuser (MD) results with and w/o SDS fitting. }
 \label{fig:fitting}
\end{center}
\end{figure*}

\begin{figure*}[t]
\begin{center}
 \includegraphics[width=\linewidth]{images/supplemental/human_mesh_generation.png}
 \caption{Human mesh generation results. }
 \label{fig:more_human}
\end{center}
\end{figure*}

\begin{figure*}[t]
\begin{center}
 \includegraphics[width=\linewidth]{images/supplemental/hand_mesh_generation.png}
 \caption{Hand mesh generation results. }
 \label{fig:more_hand }
\end{center}
\end{figure*}

\begin{figure*}[t]
\begin{center}
 \includegraphics[width=\linewidth]{images/supplemental/anima_mesh_generation.png}
 \caption{Animal mesh generation results. }
 \label{fig:more_animal}
\end{center}
\end{figure*}

\begin{figure*}[t]
\begin{center}
 \includegraphics[width=\linewidth]{images/supplemental/body_shape_variation.png}
 \caption{Body shape variation. Top: Single step approach. Feeding 3D joint locations into Mesh Diffuser as conditions and performing sampling by varying random noise,  we are able to generate meshes in different body shapes. However, this approach does not allow for the changes in body heights and segment lengths.  Bottom: Two-step approach. The first step performs unimodal generation to create a batch of skeletons with different body poses and styles and then adjusts the segment lengths of one of generated skeletons based on others in the batch. Inputting these modified skeletons into Mesh Diffuser and performing pose conditional mesh generation, we can generate meshes in diverse body styles while maintaining the pose. }
 \label{fig:more_body_shape}
\end{center}
\end{figure*}

\begin{figure*}[t]
\begin{center}
 \includegraphics[width=0.85\linewidth]{images/supplemental/interpolation.png}
 \caption{Shape interpolation results. }
 \label{fig:more_interpolation}
\end{center}
\end{figure*}

\begin{figure*}[t]
\begin{center}
 \includegraphics[width=\linewidth]{images/supplemental/refinement.png}
 \caption{Sequence of meshes constructed during shape refinement process. }
 \label{fig:more_refinement}
\end{center}
\end{figure*}

\begin{figure*}[t]
\begin{center}
 \includegraphics[width=\linewidth]{images/supplemental/control_points.png}
 \caption{Control point deformation with five control points (Wrists, ankles and head).  }
 \label{fig:more_control_points}
\end{center}
\end{figure*}

\section{Appendix: More qualitative results on 3D mesh recovery }

Figure \ref{fig:more_hmr} shows additional human mesh recovery results of Mesh Diffuser where a 3D human mesh is predicted from a single image.

\begin{figure*}[t]
\begin{center}
 \includegraphics[width=\linewidth]{images/supplemental/hmr_qualitative.png}
 \caption{Visualization of human mesh recovery results.}
 \label{fig:more_hmr}
\end{center}
\end{figure*}
